# Supplementary material for: AIOpsLab: A Holistic Framework to Evaluate AI Agents for Enabling Autonomous Clouds
Source: arXiv:2501.06706 source file (2025-01-12)
Supplement: Supplementary file 1 [file appendix.tex]

\begin{table}[t]
\caption{Other commands usage times except telemetry APIs, submit and kubectl commands.}
\label{table:other_commands}
\small
\centering
\resizebox{0.50\textwidth}{!}{%
\begin{tabular}{l|cccccccccc}
\toprule
\textbf{Agent} & \textbf{find} & \textbf{echo} & \textbf{python} & \textbf{awk} & \textbf{mongo} & \textbf{grep} & \textbf{ls} & \textbf{cat} & \textbf{ip} & \textbf{iptables} \\ \hline

\react{} & 0 & 0 & 0 & 3 & 0 & 1 & 26 & 30 & 0 & 0 \\ \hline
\tweaver{} & 5 & 1 & 10 & 6 & 0 & 3 & 40 & 57 & 1 & 1 \\ \hline
\flash{} & 0 & 3 & 0 & 0 & 0 & 0 & 8 & 10 & 0 & 0 \\ \hline
\autogen{} & 0 & 3 & 0 & 0 & 2 & 2 & 22 & 27 & 0 & 0 \\ 
\bottomrule

\end{tabular}
}
\end{table}

We also evaluate the frequency of API usage across different rounds.

\begin{figure}[htbp]
    \centering
    \subfigure[ReAct]{%
        \includegraphics[width=0.48\columnwidth]{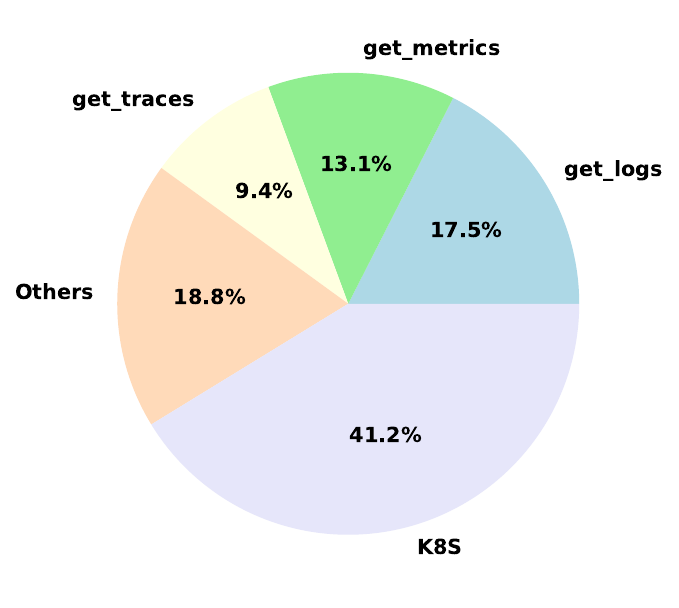}%
        \label{fig:round_pie_chart_1}
    }
    \subfigure[TaskWeaver]{%
        \includegraphics[width=0.48\columnwidth]{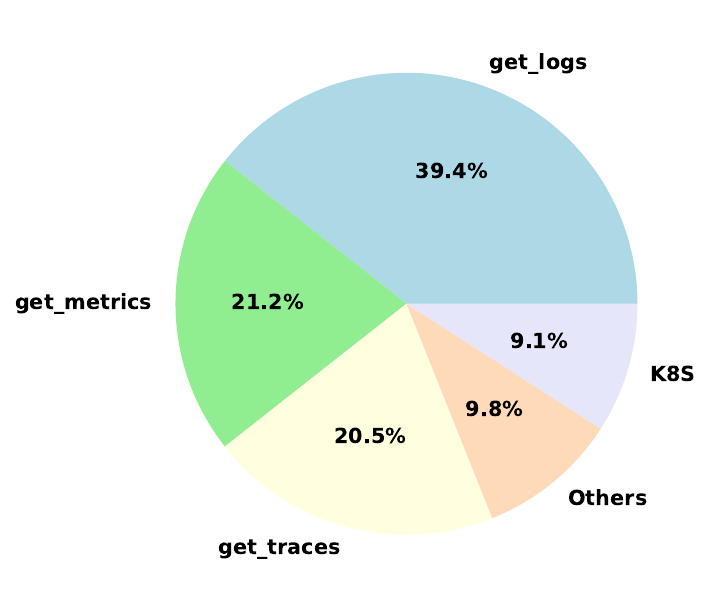}%
        \label{fig:round_pie_chart_2}
    }
    \subfigure[Flash]{%
        \includegraphics[width=0.48\columnwidth]{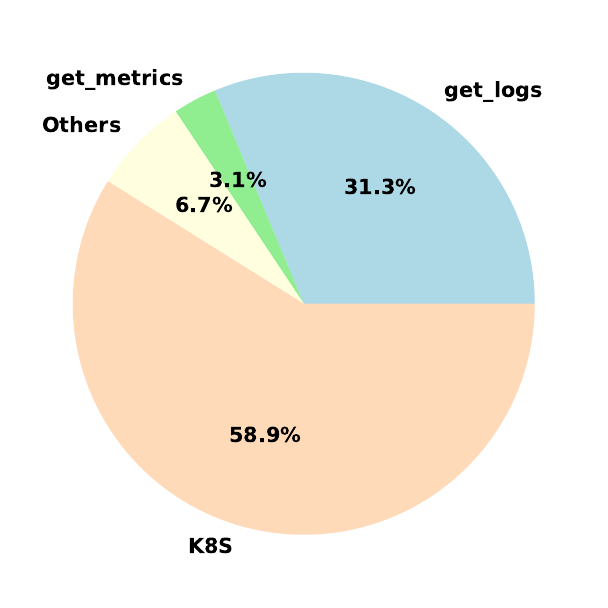}%
        \label{fig:round_pie_chart_3}
    }
    \subfigure[AutoGen]{%
        \includegraphics[width=0.48\columnwidth]{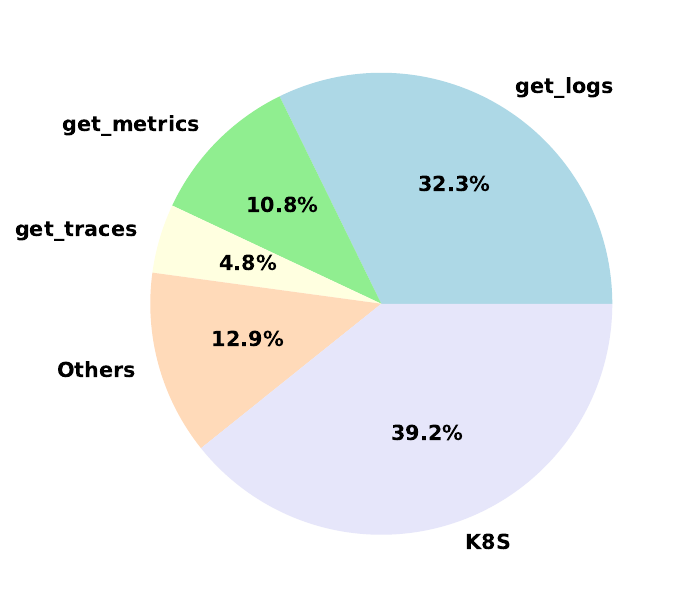}%
        \label{fig:round_pie_chart_4}
    }

    \caption{Total number of rounds for API usage.}
    \label{fig:api_charts}
\end{figure}

\yf{prompt template examples}

\yf{More agent execution traces}
